# Supplementary material for: Iterative Methods for Private Synthetic Data: Unifying Framework and New Methods
Source: arXiv:2106.07153 source file (2021-12-09)
Supplement: Supplementary file 1 [file appendix_prelims.tex]

\section{Additional Definitions}

%%%%%%%%%%%%%%%%%
%% Def 
%%%%%%%%%%%%%%%%%
\begin{definition}[R\'{e}nyi divergence,]\label{def:renyidiver}
 Let $\mu$ and $\nu$ be probability
distributions on $\Omega$. For $\alpha\in(1,\infty)$, we define the R\'{e}nyi divergence of order $\alpha$ between $\mu$ and  $\nu$ as
\begin{align*}
  \rendiver{\alpha}{\mu\parallel\nu} = \frac{1}{1-\alpha} \log \sum_{x\in\Omega} \mu(x)^\alpha\nu(x)^{1-\alpha} 
\end{align*}
\end{definition}
